# Supplementary material for: Fine structure splitting analysis of cavity-enhanced telecom-wavelength InAs quantum dots grown on a GaAs(111)A vicinal substrate
Source: arXiv:2202.11436 source file (2022-09-30)
Supplement: Supplementary file 1 [file appendix.tex]

\section{Polarisation basis and entangled states for non-collinear states}
\label{app:polarisation}
For the normal case of no magnetic field interaction, the eigenstates of the \(XX\) and \(X\) are parallel with emission of linear co-polarised photon pairs. With increasing magnetic field strength, the eigenstates of the \(XX\) and \(X\) transition to non-collinear states given by~\cite{Stevenson2011}

\begin{align}\label{eqn:wonkdot3b}
\ket{P_{XX}}  &=  \alpha \ket{H_{XX}} -i\beta\ket{V_{XX}},\\
\ket{P_{X}}  &=  \alpha \ket{H_{X}} -i\beta\ket{V_{X}}, \\
\ket{Q_{XX}}  &=  \alpha \ket{V_{XX}} -i\beta\ket{H_{XX}},\\
\ket{Q_{X}} &=  \alpha \ket{V_{X}} -i\beta\ket{H_{X}},
\end{align}
where \(\alpha^{2} + \beta^{2} = 1\) and \(\beta/\alpha = S_{c}/\left( S_{r}+S \right )\), with emission of elliptically polarised photon pairs. The two-photon state is now
\begin{equation}\label{eqn:wonkdot3}
\ket{\Psi} = \frac{1}{\sqrt{2}} \left ( \ket{P_{XX}} \ket{P_{X}}  +\allowbreak e^{i S\tau/\hbar}\ket{Q_{XX}} \ket{Q_{X}} \right ),
\end{equation}
and still results in emission of polarisation entangled photon pairs. At \(\tau=0\), the entangled state is still the expected Bell state \(\ket{\Phi^{+}}\), when expressed in the QD basis. However, for measurement of the degree of correlation in other bases, as is necessary for protocols involving entangled photon pairs~\cite{Ekert1991}, the determination of the detection basis is no longer trivial. This becomes a larger problem when considering the transmission of photons through single-mode fibre which introduces polarisation rotations and requires alignment in order to recover the states correctly~\cite{Xiang2019}.
\\
% \begin{figure}[h!]
% 	\includegraphics[width=0.45\textwidth]{Figures/wonky_dot_energy.pdf}
% 	\caption{\textbf{Modification of the polarisation eigenstates under a normally orientated magnetic field.} At zero-field, the energy structure resultant from the exchange interaction remains the same and the mixing of the  $M=\ket{\pm1}$ eigenstates results in the linearly polarised eigenbasis $\{\ket{H},\ket{V}\}$. With the application of a magnetic field in the normal direction, the eigenstates are modified resulting in an elliptically polarised non-orthogonal basis.}\label{fig:wonkyenergy}
% \end{figure}
\noindent With no magnetic field \(S_{c} \rightarrow 0\) and the states are the familiar linearly polarised state
\begin{equation}\label{eqn:wonkydot4a}
  \ket{\Psi} = \frac{1}{\sqrt{2}} \left ( \ket{H_{XX}} \ket{H_{X}}  +\allowbreak e^{i S\tau/\hbar}\ket{V_{XX}} \ket{V_{X}} \right ).
  \end{equation}
For increasing \(S_{c}\), the states become elliptically polarised before eventually tending towards the circular basis states
\begin{equation}\label{eqn:wonkydot4b}
\ket{\Psi} = \frac{1}{\sqrt{2}} \left ( \ket{R_{XX}} \ket{L_{X}}  +\allowbreak e^{i S\tau/\hbar}\ket{L_{XX}} \ket{R_{X}} \right ).
\end{equation}

\section{Fine-Structure Splitting Characterisation}
\label{app:FSS}
\noindent Polarisation-resolved spectroscopy is a convenient method to determine the FSS of neutral \(X\)s and \(XX\)s, as the polarisation of the emitted photon correlates with its energy. A polarimeter, which consists of a rotating QWP followed by fixed LP, can be used to determine this splitting through discrimination of the polarisation state of the light. If the input state of light is given in terms of Stokes parameters, the output intensity is then
\begin{align}\label{eqn:stokes}
   \begin{pmatrix}
        I_{0} \\
        I_{1} \\
        I_{2} \\
        I_{3}
    \end{pmatrix} &= \vec{M(\chi)}
    \begin{pmatrix}
        I \\
        Q \\
        U \\
        V
    \end{pmatrix},
  \end{align}
where \(I\), \(Q\), \(U\) and \(V\) denote the Stokes parameters defining the total intensity and the intensity of polarisation in the horizontal, diagonal and circular bases, respectively, \(\vec{M(\chi)}\) is the Muller matrix defining the measurement of a QWP at an angle \(\chi\) to a subsequent linear polariser \cite{Goldstein2017}, set to be aligned along the horizontal axis. The resulting measured intensity is then
\begin{equation}\label{eqn:stokes2}
    \begin{split}
    I_{0}(\chi) &= \frac{1}{2}\left(2I + Q + Q\cos(4\chi) \right.\\
    &+ \left. U\sin(4\chi) + 2V\sin(2\chi)\right).
    \end{split}
\end{equation}
This relates to the FSS, \(S\), as the mean energy, \(\langle E\rangle\), of the transition is the polarisation weighted average of the eigenstates \(\ket{X_H}\) and \(\ket{X_V}\) with energies \(E_{H} = \langle E\rangle + S/2\) and \(E_{V} = \langle E\rangle - S/2\), respectively. Thus, the energy measured by the spectrometer is then
\begin{equation}\label{eqn:stokes3}
    \begin{split}
     E_{0}(\chi) =& \frac{1}{2} \left( E_{H} \frac{I_{0}(\chi)}{I} +  E_{V} \frac{\bar{I_{0}}(\chi)}{I} \right) \\
      ={}& \frac{1}{2}\left( 2\langle E\rangle + \frac{S Q}{2I} + \frac{S Q\cos(4\chi)}{2I} \right.\\
      &+ \left.\frac{S U\sin(4\chi)}{2I} + \frac{S V\sin(2\chi)}{I} \right)
    \end{split}
\end{equation}
where \(\bar{I_{0}}(\chi)\) is the intensity of the orthogonal polarisation corresponding to \(\{Q,U,V\} \rightarrow -\{Q,U,V\}\), and \(S\) is then determined as the length of the polarised part of the energy Stokes vector
\begin{equation}\label{eqn:stokes4}
  \vec{I} = \begin{pmatrix}
        2\langle E\rangle \\
        S Q \\
        S U \\
        S V
    \end{pmatrix},
\end{equation}
following the normalisation of \(I^{2} = Q^{2} + U^{2} + V^{2} = 1\) as 
\begin{equation}
    \begin{split}
    S&=\sqrt{I^2_1 +I^2_2+I^2_3}.\\
    \end{split}
\end{equation}
This method is a reformulation of that which has been detailed in the previous work of this lab~\cite{Skiba-Szymanska2017} and is robust against fixed birefringence in the system, such as that introduced by semi-polarising optical components or optical fibre.

The added benefit of expressing the problem in this way is that we can use frequency analysis on Equation~\ref{eqn:stokes3} to directly determine the Stokes parameters in terms of the magnitude of the \(0\chi\), \(2\chi\) and \(4\chi\) frequency components by performing a Fourier Transform, allowing an essentially fitting free reconstruction of the measured polarimeter data. Analysing the data in this way is further robust to effects such as beam-steering in the intensity as this only introduces \(1\chi\) components, as long as the measurement is taken over a full rotation of the QWP.

By measuring spectra of the QD as a function of \(\chi\), \(E_{0}(\chi)\) can be calculated. As the resolution of the spectrometer grating used here is \(\sim 89\)~\(\mu\)eV, Gaussian fitting routines are required in order to accurately determine the central energy of the transition, with a resolution of approximately \(2\)~\(\mu\)eV. A Fast Fourier Transform (FFT) is then performed on the data in order to extract the relevant frequency components from which the polarimeter curve can be reconstructed.
